# Supplementary material for: Persistent control of a superconducting qubit by stroboscopic measurement feedback
Source: arXiv:1301.6095 ancillary file (2013-08-21)
Supplement: Supplementary file 1 [file supmat_campagne_PRX.pdf]

# Supplementary material for “Persistent control of a superconducting qubit by stroboscopic measurement feedback”

P. Campagne-Ibarcq,<sup>1</sup> E. Flurin,<sup>1</sup> N. Roch,<sup>1</sup> D. Darson,<sup>1</sup> P. Morfin,<sup>1</sup>

M. Mirrahimi,<sup>2</sup> M. H. Devoret,<sup>3,4</sup> F. Mallet,<sup>1</sup> and B. Huard<sup>1</sup>

<sup>1</sup>Laboratoire Pierre Aigrain, Ecole Normale Supérieure,  
CNRS (UMR 8551), Université P. et M. Curie,

Université D. Diderot 24, rue Lhomond, 75231 Paris Cedex 05, France

<sup>2</sup>INRIA Paris-Rocquencourt, Domaine de Voluceau, B.P. 105, 78153 Le Chesnay Cedex, France

<sup>3</sup>Collège de France, 11 Place Marcelin Berthelot, F-75231 Paris Cedex 05, France

<sup>4</sup>Department of Applied Physics, Yale University, PO Box 208284, New Haven, CT 06520-8284

(Dated: April 26, 2013)

## EXPERIMENTAL SETUP

### Cabling

Readout and drive pulses are generated by single side-band modulation of two continuous microwave tones produced by microwave generators set respectively at  $\omega_r/2\pi + 62.5$  MHz and  $\omega_{eg}/2\pi + 125$  MHz. The modulation is performed by mixing these tones with arbitrary shaped waveforms synthesized by a 4 channels Tektronix Arbitrary Waveform Generator. The FPGA board is a Triton-V5 VXS board by Tekmicro with one 10-bit deep input at 2.2 GSps and one 12-bit deep output at 4 GSps and the FPGA itself is a Xilinx Virtex-5. All sources are synchronized by an atomic clock, which also synchronizes the trigger of the waveform generator and the clock of the FPGA board. Both pulses

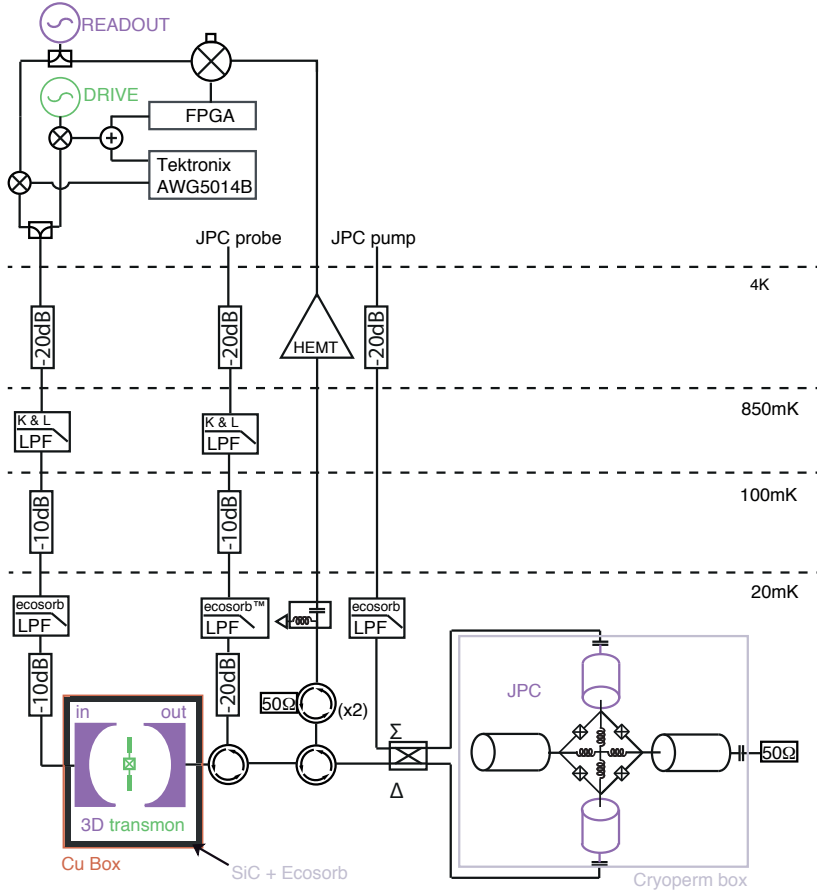

FIG. S1: Schematics of the experiment

are combined and sent towards the weakly coupled input port of the 3D aluminum cavity through an input line which is thermalized and attenuated with cryogenic attenuators at each stage of the dilution refrigerator, ensuring that only negligible thermal excitations enter the device (see Fig. S1). In particular, we took special care in terms of filtering, in order to ensure the lowest qubit thermal excitations. A commercial K&L low-pass clean-up filter of 12 GHz cut off frequency is used at the still stage (850 mK), while a home made low pass filter consisting in a microstrip line enclosed in a light tight box filled with Ecosorb (by Emerson & Cummings) is inserted at base temperature. Note that a similar line, denoted as "JPC probe" in Fig. S1, has been set up to probe the Josephson mixer, and was also used to calibrate the input and output coupling rates to the cavity  $\kappa_{in}/2\pi = 0.34$  MHz and  $\kappa_{out}/2\pi = 1.49$  MHz. Note that the internal loss rate is known to be of the order of 20 kHz which is negligible. Finally, the transmon aluminium 3D cavity is enclosed, following [1, 2], in a light tight copper box thermally anchored to the 20 mK stage. Its inside walls are all covered by a black coating consisting in 1 mm diameter SiC grains (from Saint-Gobain) mixed up in Ecosorb.

Two cryogenics circulators in series are used to direct the readout signal from the cavity to the Josephson mixer. A cryoperm magnetic shield encloses the Josephson mixer and its biasing coil (not shown). Being reflected amplified, the output signal is routed back towards a commercial HEMT amplifier of 40 dB gain from Caltech University, isolated with a bias-tee and two circulators in series. The output signal is further amplified at room temperature, mixed down by  $\omega_r$ , and amplified on a 125 MHz bandwidth. Its amplitude and phase are finally computed by an FPGA board by numerical demodulation at 62.5 MHz. Finally, by simply adjusting the phase of the modulation of the readout

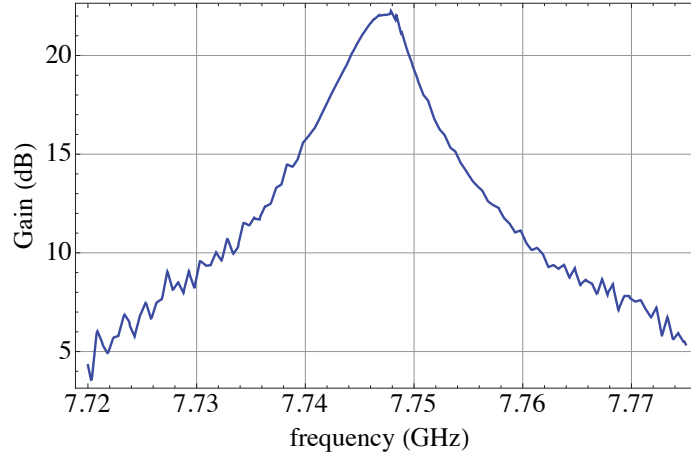

FIG. S2: Gain of the JPC as a function of frequency.

tone compared to the fixed phase of the numerical heterodyning, it is possible to align the two qubit pointer states symmetrically compared to the out-of-phase axis (see. main text Fig. 1) and thus measuring the probability of the outcome  $\text{Im}(a) > 0$  (resp.  $\text{Im}(a) < 0$ ) corresponding to the qubit in the ground state (resp. excited).

The Josephson amplifier gain was measured by turning ON and OFF the pump of the JPC. A slight shift (0.43 MHz) between the resonance frequencies of the cavity ON and OFF is likely due to imperfect isolation between the JPC and the cavity through the two circulators. A slight deterioration of coherence time due to turning on the JPC was observed in a previous similar experiment (unpublished). We therefore turn ON the JPC only during measurement times.

### Feedback delay

The FPGA board is a Tekmicro Triton-V5 board. Here, we decompose in time the various steps (see Fig. S3) contributing the total feedback delay of about 480 ns.

- 120 ns: Delay of propagation between the output of the Digital to Analog Converter (DAC) and the input of the Analog to Digital Converter (ADC) of the Triton board, when going through the cavity of the 3D Transmon. This time interval corresponds to the total electric delay of the setup.
- 180 ns: Delay of the transfer between the ADC and the FPGA itself plus the transfer between the FPGA and the DAC. This delay originates from the synchronization between the FPGA clock and the ADC/DAC clocks along the transfer. This time may be diminished at the expense of reliability.

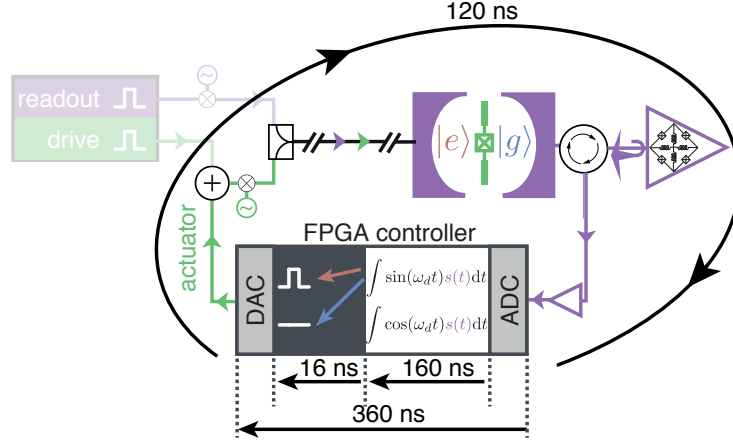

FIG. S3: Illustration of the delays added by the various steps of the feedback loop (see text).

- 160 ns: Time taken in order to finish the integration of the numerically demodulated signal after the last data sample has reached the FPGA. At the end of this delay, the averaged quadratures (non renormalized by the measurement duration) are calculated, and a bit is dedicated to the decision to apply a correcting pulse through the DAC or not.
- 16 ns: Time taken by the FPGA to send a pulse to the DAC depending on the decision bit.

## READOUT CALIBRATION

### Field amplitude inside the cavity

It is possible to calibrate *in situ* the amplitude of the field inside of the cavity during readout. When  $\kappa \approx 2\chi$ , the most reliable way to do this consists in using the measurement induced dephasing rate due to the presence of a field in the cavity. Indeed, this measurement induced dephasing rate is given by [3, 4]

$$\Gamma_m = \frac{\kappa_{tot}}{2} |\alpha_g - \alpha_e|^2, \quad (1)$$

where  $\kappa_{tot} = \kappa_{in} + \kappa_{out}$  and  $\alpha_g$  (resp.  $\alpha_e$ ) is the state of the cavity mode when the qubit is in state  $|0\rangle_q$  (resp.  $|1\rangle_q$ ). For a constant input readout power  $P_{in}$  at frequency  $\omega_r + \delta\omega$ , they read [5]

$$\alpha_g = \mu \frac{\sqrt{P_{in}}}{\kappa_{tot} - i(2\delta\omega - 2\chi)} \text{ and } \alpha_e = \mu \frac{\sqrt{P_{in}}}{\kappa_{tot} - i(2\delta\omega + 2\chi)}, \quad (2)$$

where  $\mu$  is the prefactor which needs to be calibrated.

We performed a series of Ramsey fringes measurements while varying the power  $P_{in}$  of an incoming pulse at the readout frequency during the free equatorial evolution. Starting from an empty cavity, we apply a fast  $\pi/2$  pulse (64 ns) compared to decoherence. Then, 50 ns after this rotation, a pulse 1200 ns long, with the same envelope as the one used for reading out the qubit state in the experiment, is sent at frequency  $\omega_r + \delta\omega$  with an incoming power  $P_{in}$ . Then, 2300 ns after the first  $\pi/2$  pulse, a second pulse, phase detuned by  $\phi$  from the first, is sent to rotate the qubit again. Finally, a readout pulse measuring the state of the qubit starts 50 ns after the last rotation.

This last measurement allows us to measure  $\langle \sigma_Z(\phi) \rangle$  which is a cosine function of the phase  $\phi$

$$\langle \sigma_Z(\phi, P_{in}) \rangle = A + B(P_{in}) \cos(\phi - \varphi(P_{in})). \quad (3)$$

Calling the effective measurement time  $T_{eff} \approx \int_{-\infty}^{\infty} \frac{|\alpha|^2(t)}{|\alpha_s|^2} dt$ ,  $\alpha_s$  being the stationary limit of the field amplitude  $\alpha$  in the cavity. We then have the useful relations

$$B(P_{in}) = B(0)e^{-\Gamma_m T_{eff}} \text{ and } \varphi(P_{in}) = \varphi(0) + \Delta\omega_{Stark} T_{eff}. \quad (4)$$

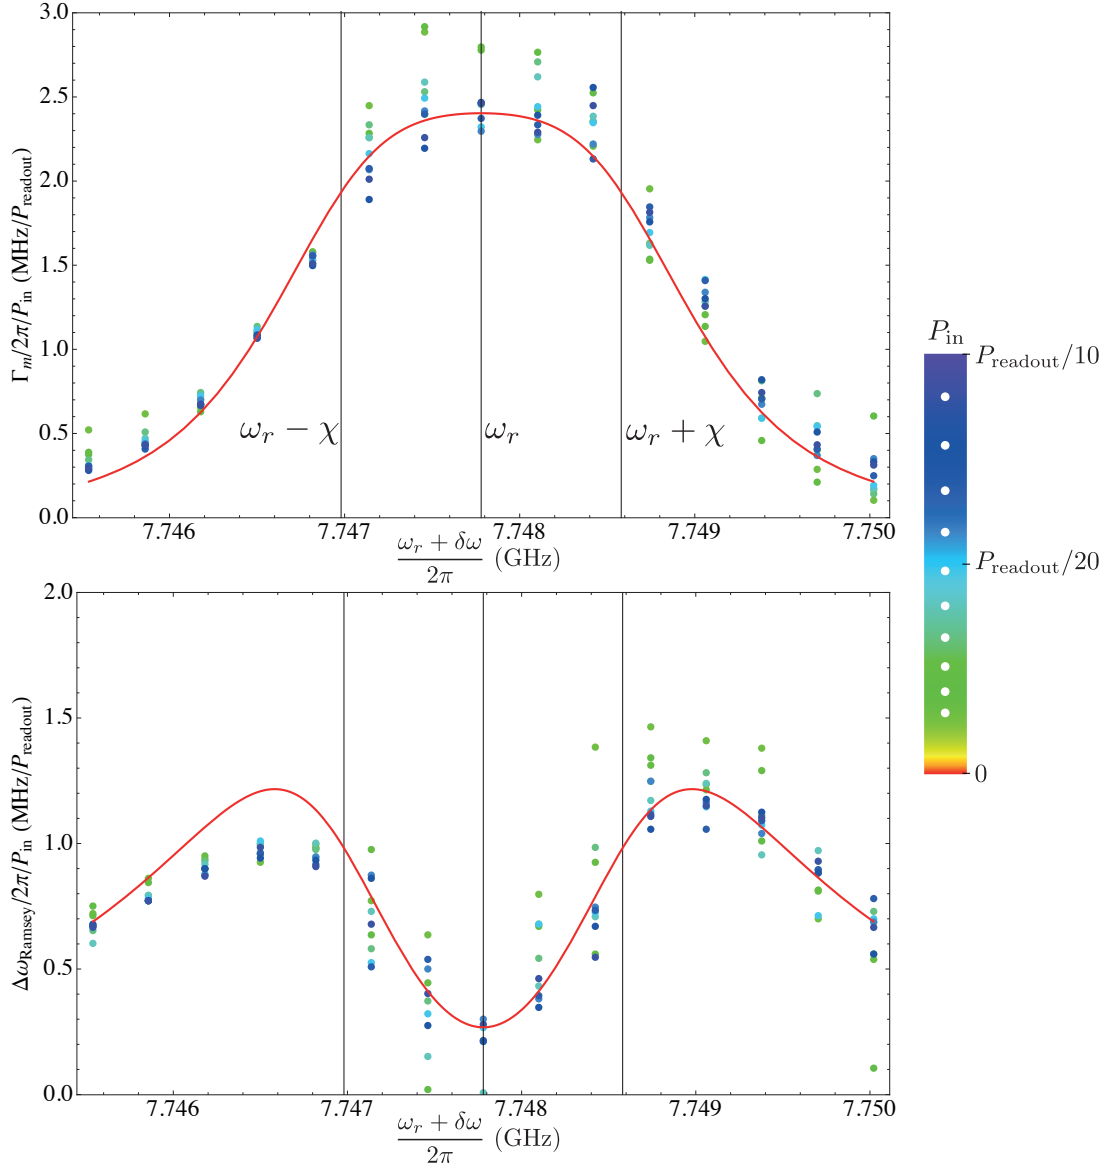

FIG. S4: (top) Dots: Measurement induced dephasing rate  $\Gamma_m$  scaled by the power of the incoming readout, which is referred to the power used for the actual readout pulses in the letter. The dephasing rate is deduced from the decay of Ramsey fringes obtained when a readout pulse, with the same duration as in the actual experiment, occurs between the two phase tuned  $\pi/2$  pulses on the qubit used for the Ramsey sequence. The contrast of the fringes is proportional to  $e^{-\Gamma_m T_{\text{eff}}}$  where the dressing power changes, with  $T_{\text{eff}} \approx \int_{-\infty}^{\infty} \frac{|\alpha|^2(t)}{|\alpha_s|^2} dt$ ,  $\alpha_s$  being the stationary limit of the field amplitude  $\alpha$  in the cavity. The measurements were performed for powers indicated by color according to the color bar. Line: theoretical expectation for the same quantity assuming a stationary number of photons equal to 1.4. (bottom) Dots: Detuning of the qubit frequency measured from the phase change of the same Ramsey fringes. Line: theoretical expectation for the same quantity assuming also 1.4 photons in the stationary limit.

On Fig. S4, we extracted the corresponding  $\Gamma_m$  and  $\Delta\omega_{\text{Stark}}$  scaled down by the power in units of the power used for the actual readout in the experiment, as a function of detuning  $\delta\omega$  for several powers ranging from  $P_{in} = 0$  to  $P_{in} = 0.2P_{in}^{\text{readout}}$ . Using the above expressions, it is easy to fit the experimental curves of Fig. S4 with  $\mu = 19 \text{ rad.s}^{-1}/\sqrt{P_{in}^{\text{readout}}}$  as a single fit parameter. We hence find a photon number during readout of  $|\alpha_g|^2 = |\alpha_e|^2 \approx 1.4$ .

According to Ref. [5], the AC-Stark shift, corresponding to the qubit frequency shift due to the irradiation of the cavity is given by

$$\Delta\omega_{\text{Ramsey}} = -2\chi \text{Re}(\alpha_e \alpha_g^*) = -2\mu^2 P_{in} \chi \frac{\kappa^2 - 4\chi^2 + \delta\omega^2}{(\kappa^2 + 4\chi^2 - \delta\omega^2)^2 + 4\delta\omega^2 \kappa^2}. \quad (5)$$

In the experiment, we perform readout pulses at  $\delta\omega = 0$  and it is interesting to note that the Stark shift goes to zero when  $2\chi \approx \kappa$  such as in our experiment. The measured AC-Stark shift is consistent with this law except close to  $\delta\omega = 0$  where the shift is not linear in power (see spread of data on Fig. S4).

### Detection efficiency

The efficiency  $\eta_{tot}$  of the detection chain can be determined from the variance of the complex field amplitude measured when the qubit is in state  $|0\rangle_q$ . The complex amplitude of each measurement pulse is determined by averaging over a measurement time  $T_{\text{meas}} = 960$  ns. Indeed, the measurement can be decomposed as  $N_m = T_{\text{meas}}\kappa_{tot} = 11.0$  temporal modes of  $|\alpha_g|^2 = 1.4$  photons each. Therefore, in the units of Fig. 1 (from main text) where the averaged field amplitude is given by  $\alpha_g$ , the variance of the measured amplitude is

$$\text{Var}(a) = \frac{1}{N_m\eta_{tot}}. \quad (6)$$

Note that this can be written also in terms of the real and imaginary parts of the field amplitude (each of variance  $1/2$  per temporal mode for  $\eta_{tot} = 1$ ) as

$$\text{Var}(\text{Re } a) + \text{Var}(\text{Im } a) = \frac{1}{N_m\eta_{tot}}. \quad (7)$$

At thermal equilibrium, the qubit is found in the ground state with a probability 98%, so that it is a very good approximation to calculate the efficiency by neglecting the other 2% events. We find  $\text{Var}(a) = 0.13$  and thus,

$$\eta_{tot} = 0.67 \quad (8)$$

A large part of the inefficiency is coming from the rather large input coupling rate. Therefore  $\eta_{tot} = \eta_{out}\eta_{det}$  where the efficiency of the extraction of radiation by the output is  $\eta_{out} = \frac{\kappa_{out}}{\kappa_{in} + \kappa_{out}} = 0.81$  and the efficiency of the detection setup is thus  $\eta_{det} = 0.82$ . Note that the quantum limited efficiency for the phase preserving detection setup is  $\eta_{det}^{(QL)} = 100$  %. The extra loss in efficiency beyond this quantum limit can be explained by an attenuation of a few dB between the cavity and the amplifier coming from insertion losses in the setup.

## READOUT ERROR AND QUBIT THERMAL EQUILIBRIUM POPULATIONS

### Readout error

Fig. S5 singles out the measured probability density  $P(\text{Im}(a))$  presented in the first figure of the article, when no drive is applied to the qubit (continuous line). For  $\text{Im}(a) < 0$ , the agreement is excellent with the predicted probability density (dotted line) using the previously discussed calibration of the readout pulse ( $N_m = 11$  temporal modes of  $|\alpha|^2 = 1.4$  photons), detection chain efficiency ( $\eta_{tot} = 67\%$ ) and dispersive shift angle ( $\theta = 40.7^\circ$ ). The readout fidelity  $\mathcal{F}$  is defined as the probability to measure  $P(\text{Im}(a)) < 0$  while the qubit is in the ground state  $|g\rangle$ , given by

$$\mathcal{F} = \frac{1}{2} \left( 1 + \text{Erf} \left( \sqrt{\eta N_m |\alpha|^2} \sin \theta \right) \right) \approx 99.8\% \quad (9)$$

### Qubit thermal equilibrium population

When no drive is applied to the qubit, we still measure a probability  $P^{th}(\text{Im}(a) > 0) = 2.4\%$  of getting an  $\text{Im}(a) > 0$  outcome. In this paragraph we demonstrate that this probability corresponds indeed to the thermal equilibrium qubit excited population  $P_{|e\rangle}^{th}$ . For that purpose, we compare the amplitude of Rabi oscillations of the qubit with and without an initial  $\pi$  pulse at the on the  $|e\rangle \leftrightarrow |f\rangle$  transition,  $|f\rangle$  being the qubit second excited state. Without this preparation pulse, the fitted amplitude of the decaying Rabi oscillation, expressed as a distance in the phase-space

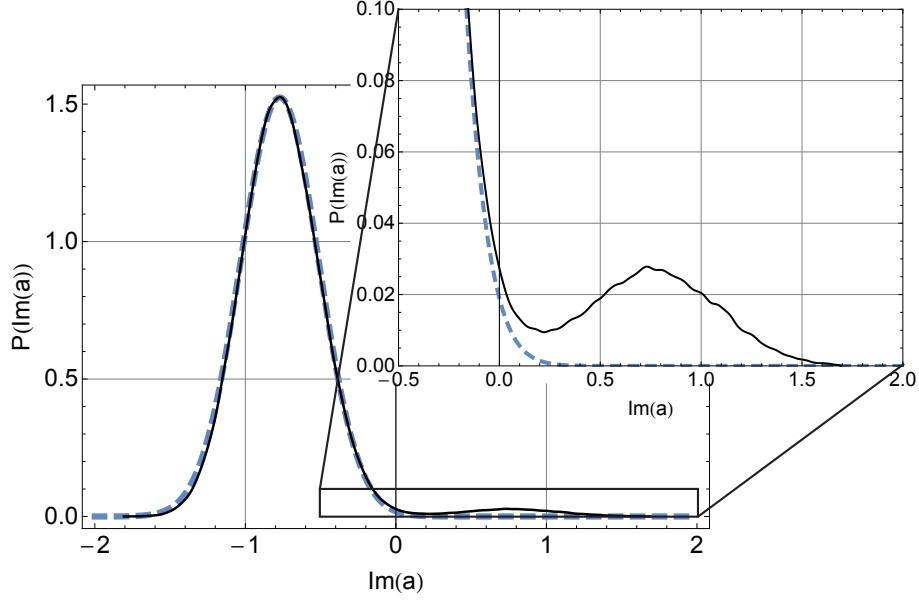

FIG. S5: Continuous (black) line: Measured probability density  $P(\text{Im}(a))$  when no drive is applied to the qubit. A thermal equilibrium probability  $P^{th}(\text{Im}(a) > 0) = 2.4\%$  of getting  $\text{Im}(a) > 0$  is observed. Dotted (blue) line: probability density of the quadrature  $\text{Im}(\alpha)$  of the inner cavity field expected from the previous calibration. The fidelity is defined as the integral of this curve on the negative half axis.

$(\text{Re}(a), \text{Im}(a))$ , is  $|\alpha_e - \alpha_g|(1 - 2P_{|e\rangle}^{th})$ . With this preparation pulse, which transfers the population  $P_{|e\rangle}^{th}$  into the second excited state, Thales intercept theorem gives a fitted amplitude of  $|\alpha_e - \alpha_g|(1 - P_{|e\rangle}^{th})$ . From the ratio of these two rabi amplitudes we obtain  $P_{|e\rangle}^{th} = 1.9\% \pm 0.3\%$ , in agreement with the measured  $P^{th}(\text{Im}(a) > 0)$  and readout error. This population corresponds to a temperature of 46 mK. Note that this number was substantially improved by a careful filtering of the microwave lines (see Fig. S1).

### Measuring of the higher excited state occupation

In order to determine an upper bound for the population in state  $|f\rangle$  at thermal equilibrium, we perform the readout pulses with a tone at  $\omega_r - \chi - 2\chi_{ef} = 2\pi \times 7.74464$  GHz, which corresponds to the maximally transmitted frequency when the qubit is in state  $|f\rangle$ . Note that  $\chi_{ef} = 1.15$  MHz is larger than  $\chi$ , contrarily to what is expected from [6]. We interpret this discrepancy by a coincidental match between upper transition frequencies of the qubit and cavity modes. We chose the phase of the field complex amplitude so that  $\text{Im}(a)$  discriminates optimally between states  $|f\rangle$  and  $|g\rangle$  or  $|e\rangle$  (see Fig. S6). Beyond a given measured value of  $\text{Im}(a)$ , the state of the qubit is  $|f\rangle$  with a large fidelity.

In the experiment, we prepare two configurations. One, at thermal equilibrium, without any pulse sequence before measurement which leads to a distribution  $P_{th}(\alpha)$  and the other with a measured distribution  $P_{\approx f}(\alpha)$ , when the qubit is prepared as close as possible to state  $|f\rangle$  in presence of relaxation. This latter state is obtained by applying a fast  $\pi$  pulse on the transition  $|g\rangle \leftrightarrow |e\rangle$ , followed by a fast  $\pi$  pulse on the transition  $|e\rangle \leftrightarrow |f\rangle$ .

In order to obtain an upper bound on the occupation  $\langle f | \rho_{th} | f \rangle$  of state  $|f\rangle$  in thermal equilibrium, we measure the likeliness  $P_s(\rho)$  to obtain  $\text{Im}(a) > s$  for a threshold  $s$  when the qubit is in state  $\rho$ . By linearity, we have

$$P_s(\rho_{th}) = \sum_{i \in \{g, e, f\}} \langle i | \rho_{th} | i \rangle P_s(|i\rangle\langle i|) \quad (10)$$

$$\geq \langle f | \rho_{th} | f \rangle P_s(|f\rangle\langle f|) \quad (11)$$

Now, using the fact the pointer state for  $|f\rangle$  has a larger imaginary part than any other pointer state at this readout frequency, we have

$$\forall s, P_s(\rho) \leq P_s(|f\rangle\langle f|),$$

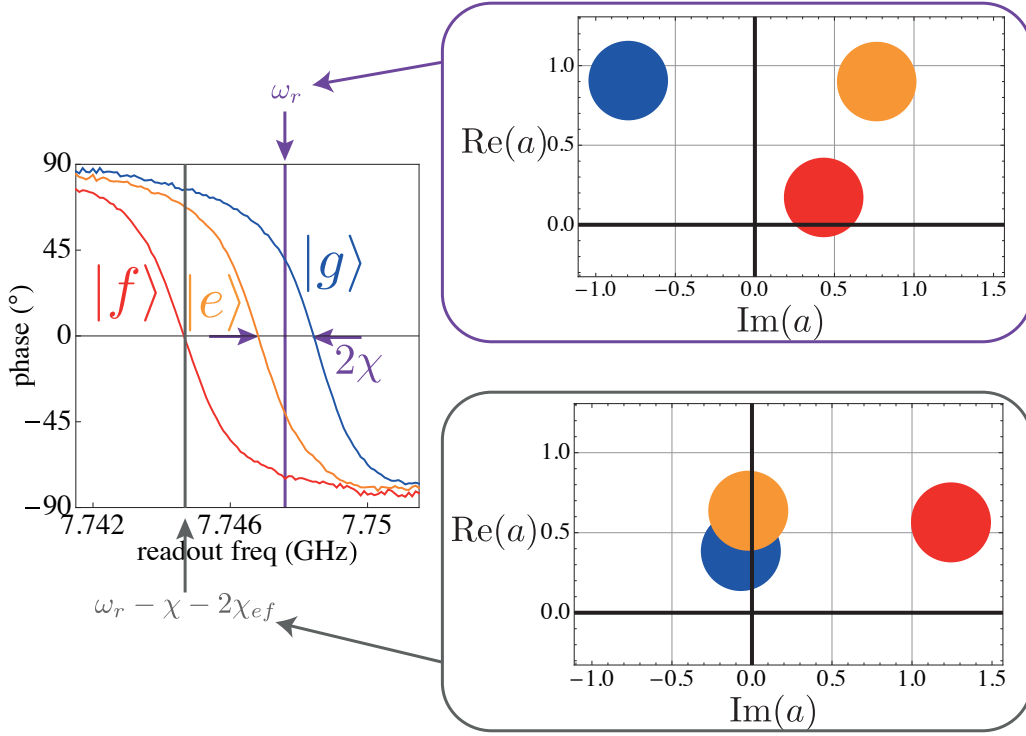

FIG. S6: (left panel) Measured phase of the transmitted signal through the cavity when the qubit is prepared in states  $|g\rangle$ ,  $|e\rangle$  or  $|f\rangle$ . (right panel) Depending on the readout frequency, the phase-preserving detection setup is able to discriminate between different states. The top panel shows the frequency used throughout the main text (optimal separation between  $|g\rangle$  and  $|e\rangle$ ) while the bottom panel shows the frequency used to measure the occupation of the  $|f\rangle$  state (see text).

and thus,

$$P_s(\rho_{th}) \geq \langle f | \rho_{th} | f \rangle P_s(\rho_{\approx f}) \quad (12)$$

There is therefore a way to give an upper bound to the occupation  $\langle f | \rho_{th} | f \rangle$  of state  $|f\rangle$  in thermal equilibrium

$$\langle f | \rho_{th} | f \rangle \leq \frac{P_s(\rho_{th})}{P_s(\rho_{\approx f})}$$

We increase this threshold  $s$  to get as strict a constraint on  $\langle f | \rho_{th} | f \rangle$  as possible while keeping enough accuracy (hence enough events). We show as a result that  $\langle f | \rho_{th} | f \rangle \leq 0.0007$ , in agreement with a thermal distribution  $\langle f | \rho_{th} | f \rangle \approx \langle e | \rho_{th} | e \rangle^2 = 0.0006$ .

## RESET BY FEEDBACK

In Fig. S7, we show the remaining population in the excited state of the qubit for four strategies of reset. Starting from the maximally mixed state (see main text), we wait for a time  $t_{\text{delay}}$  before applying 0, 1, 2 or 3 resets by feedback.

## SIMULATION OF THE TRAJECTORIES

### Rabi oscillations

We neglect here the population in states beyond  $|g\rangle$  and  $|e\rangle$  so that the evolution of the density matrix  $\rho = \begin{pmatrix} \rho_{gg} & \rho_{ge} \\ \rho_{eg} & \rho_{ee} \end{pmatrix}$  is simulated using Bloch's equations. Assuming that the qubit is driven at  $\omega_{eg}$  inducing a Rabi

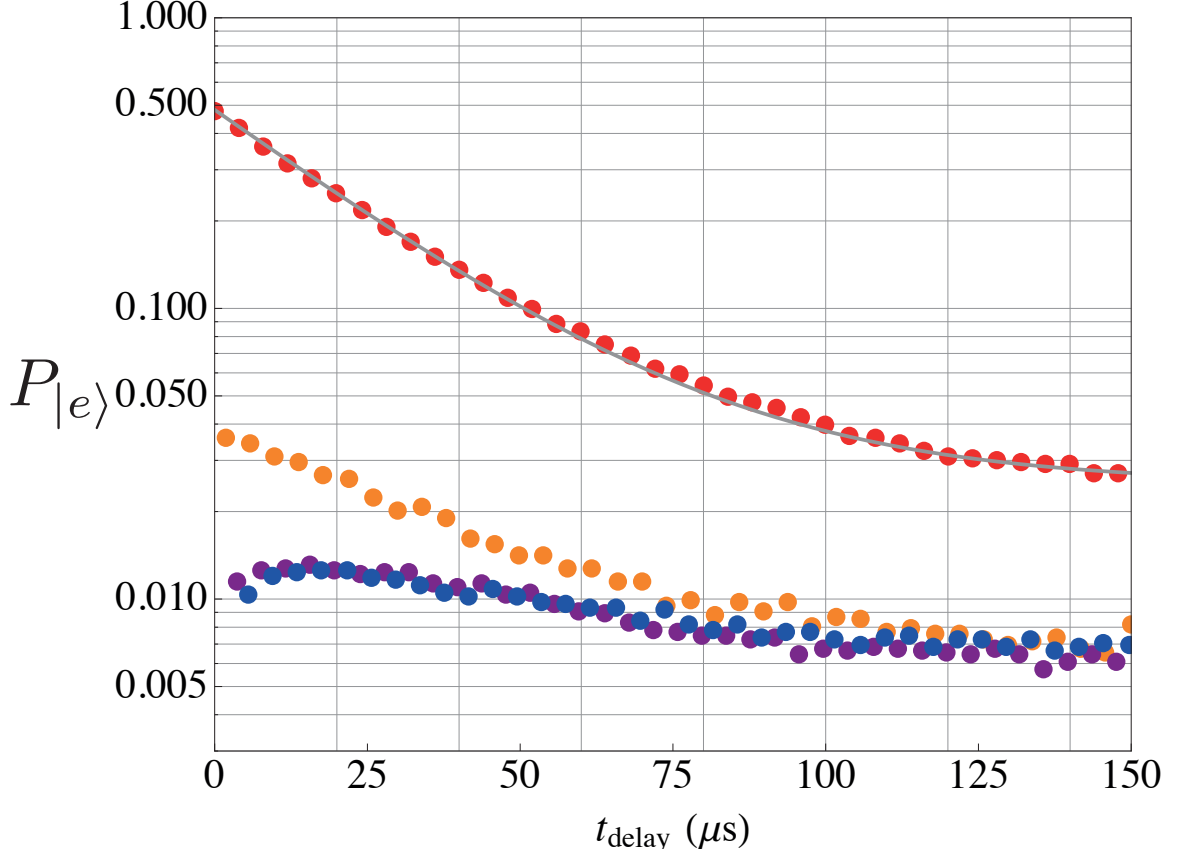

FIG. S7: Dots: Probability to measure the qubit in its excited state after a time  $t_{\text{delay}}$  for four strategies preparing the ground state  $|g\rangle$  starting from an almost perfectly mixed state. The first strategy (red) consists in simply waiting for relaxation to put the qubit into its ground state. In the second option (orange), a single measurement based reset (see Table 1 in the main text) is performed after waiting for a time  $t_{\text{delay}}$  and a  $\pi$ -pulse is then applied to the qubit in case the outcome reads  $|e\rangle$ . Another measurement at time  $t_{\text{delay}}$  then probes the efficiency of preparation of state  $|g\rangle$ . The two other options concatenate two (purple) or three (blue) feedback resets in order to improve the preparation even further. See [7] for comparison.

rotation at frequency  $\omega_R(t)$  and neglecting thermal excitations from  $|g\rangle$  to  $|e\rangle$ , these equations read

$$\frac{d}{dt} \begin{pmatrix} \rho_{ee} \\ \rho_{ge} \end{pmatrix} = \begin{pmatrix} -\Gamma_1 & \omega_R(t) \\ -\omega_R(t) & -\Gamma_2 - \Gamma_m(t) \end{pmatrix} \cdot \begin{pmatrix} \rho_{ee} \\ \rho_{ge} \end{pmatrix} + \begin{pmatrix} 0 \\ \omega_R(t)/2 \end{pmatrix} \quad (13)$$

where the time varying measurement induced dephasing  $\Gamma_m = \frac{\kappa_{tot}}{2} |\alpha_g(t) - \alpha_e(t)|^2$  (from Eq. (1)) depends on the measurement pulses. For an incoming readout pulse starting at time 0 and of duration  $\tau = 1.2 \mu s$  leading to  $\bar{n} = 1.4$  photons on average in the steady state (see Fig. S4), one can show that [8]

$$\begin{aligned} \alpha_g(t) &= -\sqrt{\bar{n}} \frac{i\sqrt{\kappa^2 + 4\chi^2}}{\kappa - 2i\chi} \left( 1 - e^{-\frac{(\kappa - 2i\chi)}{2}t} \right) & t \in [0, \tau], \\ \alpha_g(t) &= \sqrt{\bar{n}} \frac{ie^{-\frac{(\kappa - 2i\chi)}{2}t} \sqrt{\kappa^2 + 4\chi^2}}{\kappa - 2i\chi} \left( 1 - e^{\frac{(\kappa - 2i\chi)}{2}\tau} \right) & t > \tau, \\ \alpha_e(t) &= -\alpha_g^*(t). \end{aligned}$$

We can divide a period of the Rabi oscillations of length  $T_{\text{osc}} = 4000$  ns in 4 steps (see Fig. S9), each with a different driving amplitude of the qubit (and thus a different Rabi pulsation  $\omega_R$ ) and a different field amplitude the cavity.

- step A : measurement and pause from 0 to  $T_p = 1500$  ns  
During the measurement, Zeno effect prevents from performing a proper Rabi oscillation, therefore we pause

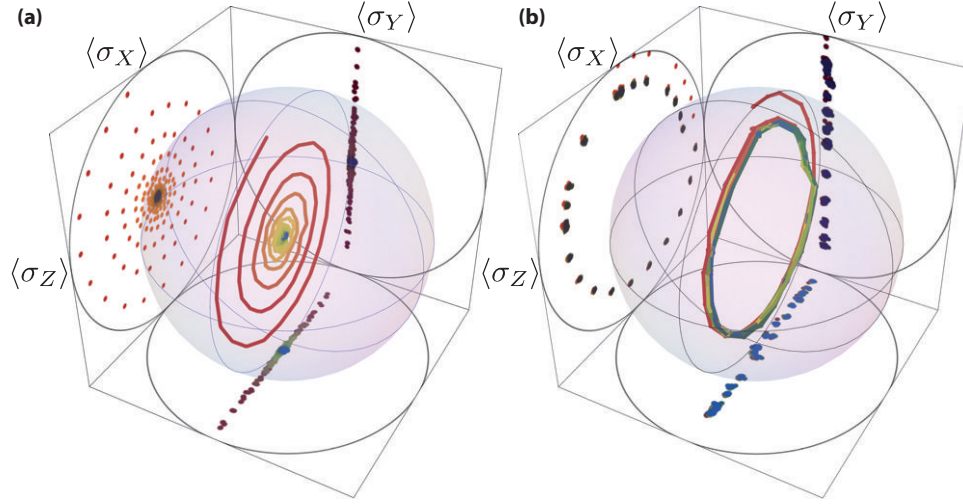

FIG. S8: (a) Decaying Rabi oscillations represented in the Bloch sphere. Here, the Rabi period is  $6.284 \mu\text{s}$  and they decay in  $T_R = 15.5 \mu\text{s}$ . The colors correspond to time as in the main text. (b) Similar representation of stabilized Rabi oscillations (Fig. 3b in the main text).

the drive power ( $\omega_R = 0$ ) as long as there is dominant measurement induced dephasing ( $\Gamma_m > 5 \Gamma_2$ ) due to the measuring field amplitude which rises inside the cavity until a steady state is reached and then, after 1200 ns, decreases during 300 ns. Coherences collapse nearly instantaneously during step A. At half the acquisition time by the FPGA board (middle of red time interval in Fig. S9), we record the population  $\rho_{ee,m}$  in  $|e\rangle$  and afterwards simulate separately two trajectories with  $\rho_{ee,m} = 0$  or  $\rho_{ee,m} = 1$  according to the measurement outcome.

- step B: fast forward from  $T_p = 1500$  ns to  $T_p + T_{\text{ff}} = 1564$  ns.  
In order to compensate for half the precession lost during the pause, the drive is performed beyond the targeted frequency during a short period of time, hence  $\omega_R = \frac{2\pi}{T_{\text{ff}}} \frac{T_p}{2T_{\text{osc}}}$  (the other half is compensated in step D). The field amplitude remaining in the cavity after step A decreases exponentially from a mean photon number 0.05 ( $\Gamma_m \simeq 5 \Gamma_2$ ) to 0.025 ( $\Gamma_m \simeq 2.5 \Gamma_2$ ). In fact, the JPC is turned off after the measurement and there may be a change in the effective cavity exit rate  $\kappa_{\text{tot}}$  in time or effective measurement duration. A slight modification of these parameters allow a much better fit to the measured trajectory.
- step C : nominal Rabi drive from  $T_p + T_{\text{ff}} = 1564$  ns to  $T_{\text{osc}} - T_{\text{ff}} = 3936$  ns.  
Rabi oscillation is here nominally driven at the target frequency  $\omega_R = \frac{2\pi}{T_{\text{osc}}}$ . Average photon number in the cavity keeps decreasing down to 0. At  $t = 1850$  ns, a correcting  $\pi$ -pulse occurs in case the previous measurement outcome is  $|e\rangle$ . We therefore add up, in the simulation, the two parallel trajectories simulated during step A, with weights  $\rho_{ee,m}$  (qubit measured in  $|e\rangle$ ) and  $1 - \rho_{ee,m}$  (qubit measured in  $|g\rangle$ ). To take into account the finite fidelity of the measurement, the first trajectory receives a correcting pulse with probability  $\mathcal{F} = 0.998$  and the second one with a probability  $1 - \mathcal{F} = 0.002$  (see section on measurement fidelity).
- step D : fast forward from  $T_{\text{osc}} - T_{\text{ff}} = 3936$  ns to  $T_{\text{osc}} = 4000$  ns.  
Same purpose as step B with  $\omega_R = \frac{2\pi}{T_{\text{ff}}} \frac{T_p}{2T_{\text{osc}}}$ . There is no readout field inside the cavity at this step.

For any initial value of  $\rho$ , the trajectory converges in about 3 or 4 periods toward the steady state represented in Fig. S9.

### Ramsey oscillations

The strategy for simulating Ramsey oscillations is very similar to this one. The fast-forward steps B and C are replaced by 64 ns long  $\pm\pi/2$  pulses and there is no drive during step C. At time 0 in the simulation, the qubit is rotated towards state  $(|g\rangle + |e\rangle)/\sqrt{2}$ .

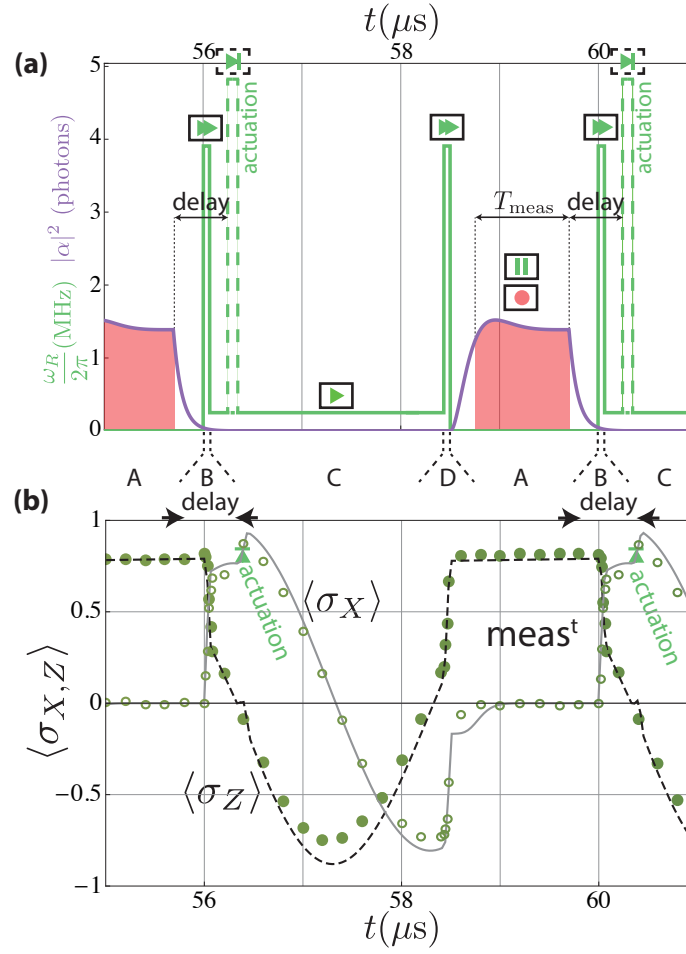

FIG. S9: (a) Pulse sequence for stabilizing Rabi oscillations. For a typical period of  $4 \mu s$ , the lines represent the drive amplitude (green) and expected occupation of the cavity (purple). The complex amplitude  $a$  of the measurement field is recorded only during the steady part of the occupation (red area). When  $\text{Im}(a) > 0$ , a fast  $\pi$  pulse is applied after a total delay of 500 ns (actuation). (b) Persistent Rabi oscillations measured using the pulse sequence described in (a) represented in  $\langle \sigma_Z \rangle$  (dots) and  $\langle \sigma_X \rangle$  (circles). The simulation result is shown as lines, dashed for  $\langle \sigma_Z \rangle$  and gray for  $\langle \sigma_X \rangle$ .

- 
- [1] R. Barends, J. Wenner, M. Lenander, Y. B. Chen, J. Kelly, E. Lucero, P. O'Malley, M. Mariantoni, D. Sank, et al., Appl. Phys. Lett. **99**, 113507 (2011), URL <http://dx.doi.org/10.1063/1.3638063>.
  - [2] A. D. Corcoles, J. M. Chow, J. M. Gambetta, C. Rigetti, J. R. Rozen, G. A. Keefe, M. B. Rothwell, M. B. Ketchen, and M. Steffen, Appl. Phys. Lett. **99**, 181906 (2011), URL <http://dx.doi.org/10.1063/1.3658630>.
  - [3] D. I. Schuster, A. Wallraff, A. Blais, L. Frunzio, R.-S. Huang, J. Majer, S. M. Girvin, and R. J. Schoelkopf, Phys. Rev. Lett. **94**, 123602 (2005), URL <http://link.aps.org/doi/10.1103/PhysRevLett.94.123602>.
  - [4] F. R. Ong, M. Boissonneault, F. Mallet, A. Palacios-Laloy, A. Dewes, A. C. Doherty, A. Blais, P. Bertet, D. Vion, and D. Esteve, Phys. Rev. Lett. **106**, 167002 (2011), URL <http://link.aps.org/doi/10.1103/PhysRevLett.106.167002>.
  - [5] J. Gambetta, A. Blais, D. I. Schuster, A. Wallraff, L. Frunzio, J. Majer, M. H. Devoret, S. M. Girvin, and R. J. Schoelkopf, Phys. Rev. A **74**, 042318 (2006), URL <http://link.aps.org/doi/10.1103/PhysRevA.74.042318>.
  - [6] S. E. Nigg, H. Paik, B. Vlastakis, G. Kirchmair, S. Shankar, L. Frunzio, M. H. Devoret, R. J. Schoelkopf, and S. M. Girvin, Phys. Rev. Lett. **108**, 240502 (2012), URL <http://link.aps.org/doi/10.1103/PhysRevLett.108.240502>.
  - [7] D. Riste, C. C. Vultink, K. W. Lehnert, and L. Dicarlo, arXiv **quant-ph**, 1207.2944v1 (2012), URL <http://arxiv.org/abs/1207.2944v1>.
  - [8] M. Mirrahimi, B. Huard, and M. H. Devoret, in Proceedings of the 51st IEEE Conference on Decision and Control (2012).
